# Supplementary material for: Improving the prediction of glassy dynamics by pinpointing the local cage
Source: arXiv:2301.13106 ancillary file (2023-01-30)
Supplement: Supplementary file 1 [file SI.pdf]

# Supplementary information: Improving the prediction of glassy dynamics by pinpointing the local cage

Rinske M. Alkemade,[1] Frank Smallenburg,[2] and Laura Filion[1]
[1)] *Soft Condensed Matter, Debye Institute of Nanomaterials Science, Utrecht University, Utrecht, Netherlands*
[2)] *Université Paris-Saclay, CNRS, Laboratoire de Physique des Solides, 91405 Orsay, France*

## I. STRUCTURAL ORDER PARAMETERS

To characterize the local environment of particles, we use the recursive structural order parameters described in Ref. 1. In particular, we use parameters that capture both the local density as well as the local $n$-fold symmetry. The local density is measured by using radial density functions that capture the density in a shell at distance $r$ and with thickness $2\delta$ from the reference particle. The local density is defined as,

$$G_i^{(0)}(r,\delta,s) = \sum_{j\neq i, s_j=s} e^{-\frac{(r_{ij}-r)^2}{2\delta^2}}, \tag{S1}$$

where $i$ is the reference particle and $r_{ij}$ is the absolute distance between particles $i$ and $j$. Note that the sum is particle type specific, it only sums over all other particles $j$ in the system that are part of particle species $s$.

To capture the local symmetry at a distance $r$ as seen from the reference particle, we first compute the complex coefficient

$$q_i^{(0)}(l,m,r,\delta) = \frac{1}{Z}\sum_{i\neq j} e^{-\frac{(r_{ij}-r)^2}{2\delta^2}} Y_l^m(\mathbf{r}_{ij}). \tag{S2}$$

Here $Y_l^m(\mathbf{r}_{ij})$ is the $l^{\text{th}}$ spherical harmonic function and $m$ is an integer that runs from $-l$ to $l$. Additionally, $Z$ is given by

$$Z = \sum_{i\neq j} e^{-\frac{(r_{ij}-r)^2}{2\delta^2}}. \tag{S3}$$

Similar to the radial density, mainly particles that are within the shell $r-\delta$ to $r+\delta$ contribute to $q_i^{(0)}(l,m,r,\delta)$. Finally, we sum over all possible values of $m$ to obtain the rotationally invariant structural parameters:

$$q_i^{(0)}(l,r,\delta) = \sqrt{\frac{4\pi}{2l+1}\sum_{m=-l}^{m=l} |q_i^{(0)}(l,m,r,\delta)|^2}. \tag{S4}$$

Below we will specify per system for which values of $r$, $\delta$ and $l$ these functions are evaluated.

### 1. Zeroth order descriptors

The radial functions are evaluated for up to 5 shells of particles as seen from the reference particle, whereas the bond order parameters are evaluated for up to 2 shells for $l \in [1, 12]$. See Fig. S1 for the pair correlation functions and the corresponding minima of the different systems. The $r$-spacing and the corresponding $\delta$-values are chosen small for small $r$, and larger for larger $r$.

For our three systems, we thus obtain the following set of $0^{th}$ order parameters.

- HS (306 parameters in total)
  - 162 radial functions with $s \in A, B$:
    - ∗ 46 equally spaced in the interval $r/\sigma_A \in (0.85, 2.0]$ with $\delta/\sigma_A = 0.025$.
    - ∗ 20 equally spaced in the interval $r/\sigma_A \in (2.0, 3.0]$ with $\delta/\sigma_A = 0.050$.
    - ∗ 15 equally spaced in the interval $r/\sigma_A \in (3.0, 4.5]$ with $\delta/\sigma_A = 0.100$.

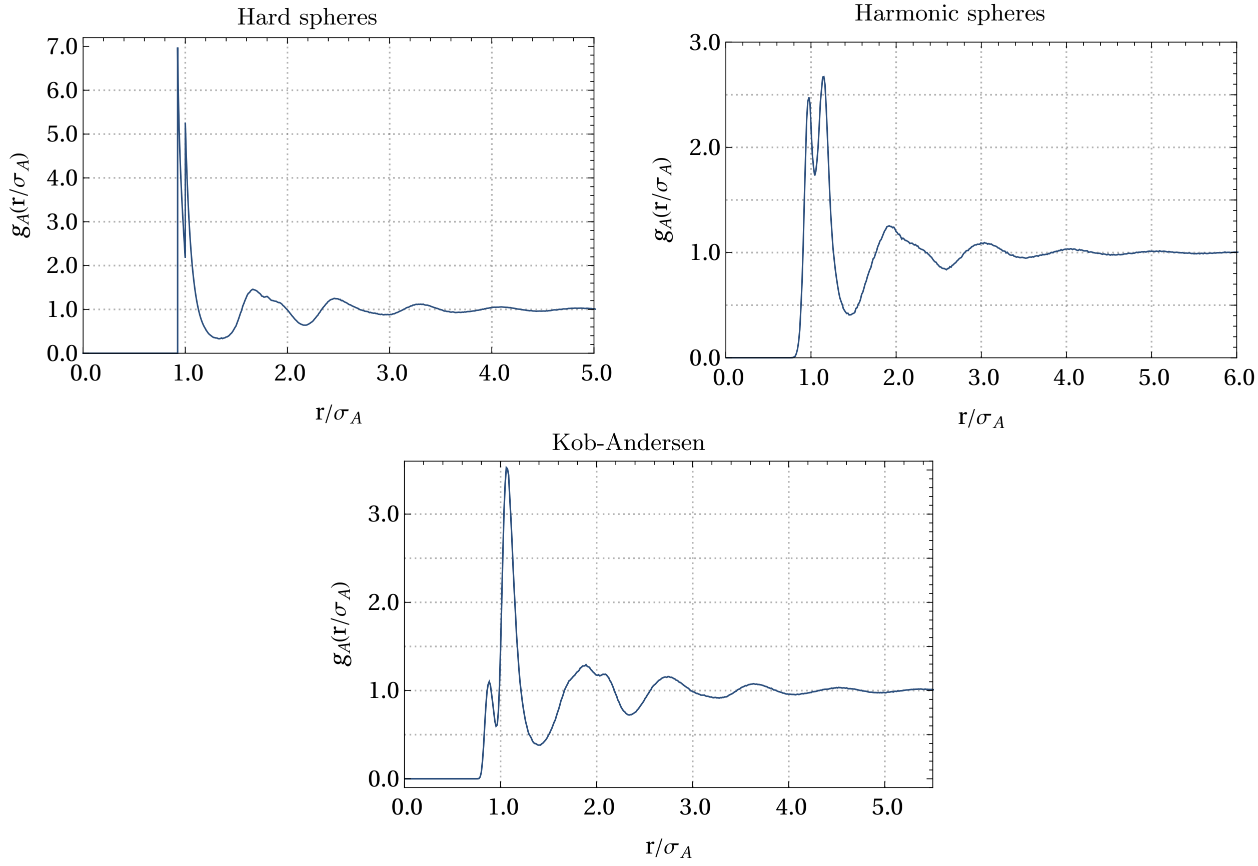


FIG. S1. Pair correlation for the $A$ particles for the three different systems (hard-sphere mixture, harmonic mixture and Kob-Andersen mixture).

  - 144 Angular fuctions
    * 12 equally spaced in the interval $r/\sigma_A \in [1.0, 2.1]$ with $\delta/\sigma_A = 0.1$ and $l \in [1, 12]$

- harmonic (428 parameters in total)
  - 212 radial functions with $s \in A, B$:
    * 60 equally spaced in the interval $r/\sigma_A \in (0.5, 2.0]$ with $\delta/\sigma_A = 0.025$.
    * 20 equally spaced in the interval $r/\sigma_A \in (2.0, 3.0]$ with $\delta/\sigma_A = 0.050$.
    * 26 equally spaced in the interval $r/\sigma_A \in (3.0, 5.6]$ with $\delta/\sigma_A = 0.100$.
  - 216 Angular fuctions
    * 18 equally spaced in the interval $r/\sigma_A \in [1.0, 2.7]$ with $\delta/\sigma_A = 0.1$ and $l \in [1, 12]$

- KA (366 parameters in total)
  - 198 radial functions with $s \in A, B$:
    * 60 equally spaced in the interval $r/\sigma_A \in (0.5, 2.0]$ with $\delta/\sigma_A = 0.025$.
    * 20 equally spaced in the interval $r/\sigma_A \in (2.0, 3.0]$ with $\delta/\sigma_A = 0.050$.
    * 19 equally spaced in the interval $r/\sigma_A \in (3.0, 4.9]$ with $\delta/\sigma_A = 0.100$.
  - 168 Angular fuctions
    * 14 equally spaced in the interval $r/\sigma_A \in [1.0, 2.3]$ with $\delta/\sigma_A = 0.1$ and $l \in [1, 12]$

### A. Higher-order structural order parameters

To calculate the higher-order generations of order parameters, we again follow Ref. 1, and define:

$$x_i^{(n)} = \frac{\sum_{j:r_{ij}<r_{\text{cut}}} x_j^{(n-1)} e^{-r_{ij}/r_{\text{cut}}}}{\sum_{j:r_{ij}<r_{\text{cut}}} e^{-r_{ij}/r_{\text{cut}}}}. \tag{S5}$$

Here $x_i^{(n)}$ are the structural parameters (which can be both radial density or bond order parameters) of order $n$ for particle $i$. The sum goes over all particles within a certain radius $r_{\text{cut}}$ as seen from the reference particle $i$. This $r_{\text{cut}}$ is chosen to be located at the second minimum of the radial distribution function, corresponding to $r_{\text{cut}}^{\text{HS}} = 2.1\sigma_A$, $r_{\text{cut}}^{\text{harmonic}} = 2.7\sigma_A$ and $r_{\text{cut}}^{\text{KA}} = 2.3\sigma_A$ for respectively the binary hard-spheres mixture, the binary harmonic mixture and the binary Kob-Andersen mixture. Note that for each model, we consider up to two generations (in addition to generation 0), and hence our total set of structural descriptors $\mathbf{X}$ consists of three times the number of parameters in the zeroth generation for each model.

## II. CAGE CENTER PREDICATION VIA SPHERICAL CONFINEMENT

In the main text, we restrict the position of particles to their approximate Voronoi cages to find the cage state. Although this method turns out to work very well, it is not the only approach possible. As an alternative, we also tried restricting the positions of particles to a sphere with a radius $r_c$ centered on their initial position. Below we will briefly discuss the findings.

In order to account for the different particle sizes, we choose $r_c^i = c \cdot \sigma_i/2$, where $\sigma_i$ is the diameter of particle $i$ and $c$ is a constant. Note that we again set $\sigma_i = \sigma_{ii}$ for all models. To compare the two methods, we again look at the correlation between the dynamic propensity and $\Delta r^{\text{cage}} = |\mathbf{r}^{\text{cage}} - \mathbf{r}^{\text{init}}|$. In the case of spherical confinement, the results depend on the value of $c$. In Fig. II we show the correlations between the dynamic propensity and $\Delta r_{\text{cage}}$ for different choices of $c$. As a reference, we also plot the correlation between the dynamic propensity and $\Delta r_{\text{cage}}$ found with the Voronoi method. In this figure we can see that the peak in the correlation moves monotonically to later times as we increase $c$. This result is not very surprising; for low values of $c$ particles that start very far from their equilibrium position will not be able to reach their cage position, while for large $c$ particles will sometimes be able to move past each other and thus escape their cage.

As we can see, the values of $c$ that yield the highest peak are close to 1, i.e. when the particle is more or less restricted to its own radius. Moreover, in all three cases we see that the curve for $c = 1.25$ lies extremely close to the one obtained using the Voronoi method. This is understandable, since the Voronoi cell of each particle is slightly larger than the volume of the particle itself.

For the hard-sphere system, we also explore how the propensity predictions change when the linear regression model is trained on the configuration found with $c = 1$, instead of the configuration found with the Voronoi method. In Fig. S3 we show the results. The panel on the left contains the propensity predictions based on the structural parameters based on the initial configuration, the configuration found with the Voronoi method and the configuration found with $c = 1$ restriction. As we can see, the difference between the two restriction methods is almost negligible. In the panel on the right, we show the correlations based on the set of input parameters given by $\mathbf{X}^{\text{init}}$ and by $\{\mathbf{X}^{\text{init}}, \mathbf{X}^{\text{CS}}, \Delta r^{\text{CS}}\}$. As we can see, the behavior is again very similar, with the only difference being a slight shift of the peak in the correlations during the caging regime to shorter times. In short, although there are small differences in the final predictions, the spherical and Voronoi confinement methods are equally effective.

## REFERENCES

[1] E. Boattini, F. Smallenburg, and L. Filion, "Averaging local structure to predict the dynamic propensity in supercooled liquids," Phys. Rev. Lett. **127**, 088007 (2021).

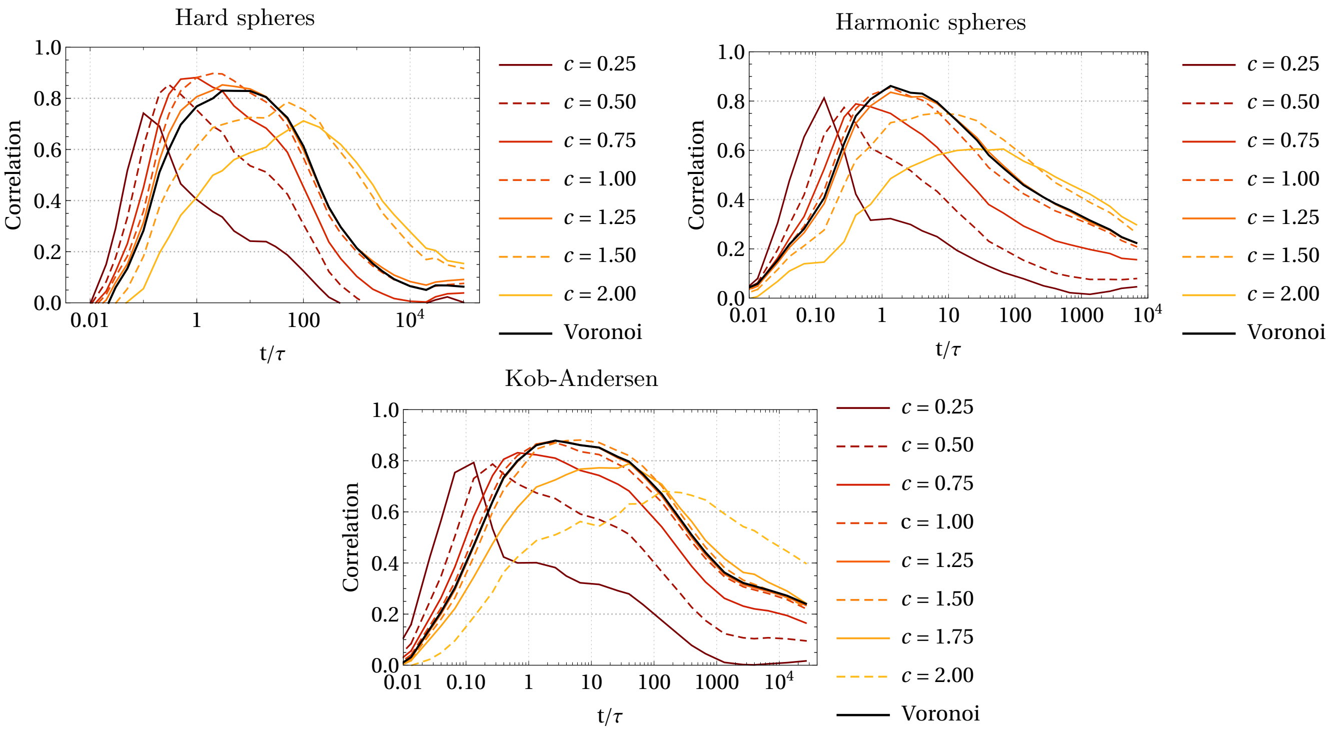


FIG. S2. Correlation between cage center and dynamic propensity as a function of time. Differently colored lines correspond to different restriction radii used during the simulations performed to obtain the cage state. Black lines correspond to the Voronoi method. Note that results are only shown for A particles. Also note that for the Kob-Anderson model, the lines for the Voronoi method and for $c = 1.25$ are essentially the same.

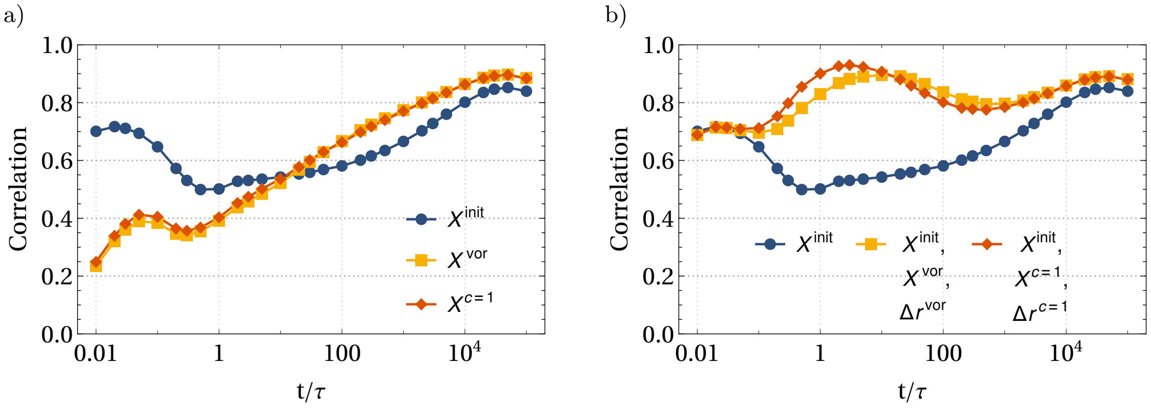


FIG. S3. **a)** Pearson correlation coefficient between the dynamic propensity and the prediction of a linear regression model trained on the structural parameters evaluated for the initial state ($\mathbf{X}^{\text{init}}$) and the cage-state coordinates evaluated with either the Voronoi restriction method ($\mathbf{X}^{\text{vor}}$) or the spherical confinement method with $c = 1$ ($\mathbf{X}^{c=1}$). Note that we consider A particles in a hard-sphere system. **b)** Correlation between the measured propensity and the predicted propensity by a linear regression model trained on either only the structural parameters based on the initial positions, or the set of input parameters given by $\{\mathbf{X}^{\text{init}}, \mathbf{X}^{\text{vor/c=1}}, \Delta r^{\text{vor/c=1}}\}$.
